# Supplementary material for: Stable Configurations Of Charged Sedimenting Particles
Source: arXiv:1810.02640 ancillary file (2018-10-08)
Supplement: Supplementary file 1 [file SupplementalMaterial.pdf]

# Stable Configurations Of Charged Sedimenting Particles: Supplemental Material

C I Trombley & M L Ekiel-Jeżewska
Institute of Fundamental Technological Research,
Polish Academy of Sciences,
Pawińskiego 5b, 02-106 Warsaw, Poland

## 1 Searching For Feasible Stable Stationary States When Particle 2 Is Not More Dense Than The Surrounding Fluid

In the text we assumed that the reduced mass $m_2$ of particle 2 was greater than zero - i.e. particle 2 was more dense than the fluid. In this section, we will examine the dynamics for $m_2 \leq 0$. When particle 2 is not more dense than the fluid, the normalization scheme used in the text is not applicable because the characteristic velocity scale must be positive and finite. We now will consider four remaining cases: Case 1 $m_2 \leq 0$ & $m_1 < 0$, Case 2 $m_2 < 0$ & $m_1 \geq 0$, Case 3 $m_2 = 0$ & $m_1 > 0$ and Case 4 $m_1 = m_2 = 0$.

Table 1: We summarize our results in this table. First we show whether there exist feasible stable stationary state. Next, we give where to find a proof.

| | | $m_2$ | | |
|---|---|---|---|---|
| | | <0 | =0 | >0 |
| $m_1$ | <0 | Yes: Case 1 | No: Case 1 | No: Main Text |
| | =0 | No: Case 2 | No: Case 4 | No: Main Text |
| | >0 | No: Case 2 | No: Case 3 | Yes: Main Text |

### Case 1: $m_2 \leq 0$ & $m_1 < 0$

We choose our new characteristic velocity as follows:

$$V' = -\frac{m_1 g}{6\pi\mu L} \tag{S.1}$$

And choose our non-dimensional parameters to be

$$\gamma' = \frac{a_2}{a_1} \tag{S.2}$$

$$\delta' = \frac{m_2}{m_1} \tag{S.3}$$

$$\beta' = \frac{kq_1q_2}{L^2 m_1 g} \tag{S.4}$$

This makes the dynamics of the system evolve according to the non-dimensional ordinary differential equation

$$\begin{aligned}\dot{\boldsymbol{\alpha}} &= \frac{3}{2|\boldsymbol{\alpha}|^3}\beta' \boldsymbol{\mathcal{G}} \cdot \boldsymbol{\alpha} + \frac{3}{4}(1-\delta')\, \boldsymbol{\mathcal{G}} \cdot \hat{\mathbf{z}} - \beta' \frac{(1+\gamma')^2}{\gamma'|\boldsymbol{\alpha}|^3}\boldsymbol{\alpha} \\ &- \frac{(\gamma'-\delta')(1+\gamma')}{\gamma'}\hat{\mathbf{z}}\end{aligned} \tag{S.5}$$

This equation is formally the same as the original equation (9), so the analysis can be repeated in exactly the same way as in the text with the appropriate reinterpretation of parameters. In particular, there exist feasible stable stationary state with the conditions analogous to those in the main text.

We can derive $\beta' > 0$ & $\delta' > 0$ as necessary conditions for stability as in the main text. This rules out feasible stable stationary states when $m_2 = 0$ & $m_1 < 0$. There can exist feasible stable stationary states when $m_2 < 0$ & $m_1 < 0$ and the charges are opposite in sign. In fact, there is a one-to-one correspondence between the feasible stable stationary states in the $m_2 < 0$ & $m_1 < 0$ case and those that exist in the main text - i.e. in the $m_2 > 0$ & $m_1 > 0$ case. In both cases, particle 2 is "above" particle 1 with respect to the sum of gravitational and buoyancy force.

## Case 2: $m_2 < 0$ & $m_1 \geq 0$

If particle 2 is less dense than the fluid and particle 1 not less dense - then there again needs to be a change of parameters. We choose our new characteristic velocity and characteristic force ratio:

$$V'' = -\frac{m_2 g}{6\pi\mu L} \tag{S.6}$$

$$\beta'' = \frac{kq_1q_2}{L^2 m_2 g} \tag{S.7}$$

And choose the other parameters as before. We now get

$$\dot{\boldsymbol{\alpha}} = \frac{3}{2|\boldsymbol{\alpha}|^3}\beta'' \boldsymbol{\mathcal{G}} \cdot \boldsymbol{\alpha} - \frac{3}{4}(1-\delta)\, \boldsymbol{\mathcal{G}} \cdot \hat{\mathbf{z}} - \beta'' \frac{(1+\gamma)^2}{\gamma|\boldsymbol{\alpha}|^3}\boldsymbol{\alpha} + \frac{(\gamma-\delta)(1+\gamma)}{\gamma}\hat{\mathbf{z}} \tag{S.8}$$

The stability conditions for this differential equation can be worked out as in the main text. It will now be shown that there is no feasible stable stationary state in this case. This will be a proof by contradiction. We start by finding the conditions analogous to equation and inequalities (14) - (17) for our new equation. The new dynamics will be of the form

$$\dot{\epsilon} = G(\alpha)\epsilon \tag{S.9}$$

$$\dot{\alpha} = F(\alpha) \tag{S.10}$$

where $G$ is analogous to $g$ in (12) and $F$ is analogous to $f$ in (13). Explicitly:

$$G(\alpha) = \frac{12\gamma\beta'' - 4(1+\gamma)^2\beta''\alpha - 3\gamma(1-\delta)\alpha^2}{4\gamma\alpha^4} \tag{S.11}$$

$$F(\alpha) = \frac{6\gamma\beta'' - 2(1+\gamma)^2\beta''\alpha - 3\gamma(1-\delta)\alpha^2 + 2(\gamma-\delta)(1+\gamma)\alpha^3}{2\gamma\alpha^3} \tag{S.12}$$

Just as before, the necessary and sufficient conditions for a feasible vertical asymptotically stable stationary state are

$$F(\alpha^*) = 0 \tag{S.13}$$

$$G(\alpha^*) < 0 \tag{S.14}$$

$$F'(\alpha^*) < 0 \tag{S.15}$$

$$1 < \alpha^* \tag{S.16}$$

The first task is showing that if such an $\alpha^*$ obtains, then $\beta'' > 0$. Exactly as (18) in the main text, we get

$$\frac{3\beta''}{\alpha^{*3}} = 3F(\alpha^*) - \alpha^*(2G(\alpha^*) + F'(\alpha^*)) > 0 \tag{S.17}$$

Where the last inequality comes from combining all four conditions (S.13) - (S.16). By (S.16), this entails $\beta'' > 0$.

Next we partition equation (S.13) into $0 = 2\gamma\alpha^{*3}F(\alpha^*) = \frac{2}{3}\gamma\alpha^{*4}F'(\alpha^*) + r_1(\alpha^*) + r_2(\alpha^*)$ where $r_1(\alpha^*) = -\gamma(1-\delta)\alpha^{*2}$ and $r_2(\alpha^*) = -\frac{2}{3}\beta''(2(1+\gamma)^2\alpha^* - 9\gamma)$. Notice that, since $\gamma > 0$ and $\delta < 0$, $r_1 < 0$. This and (S.15) imply $r_2 > 0$, therefore

$$\alpha^* < \frac{9}{2}\frac{\gamma}{(1+\gamma)^2} < \frac{9}{8} \tag{S.18}$$

This also gives us a bound on $\gamma$

$$\frac{1}{2} < \gamma < 2 \tag{S.19}$$

We will now derive a bound on $1-\delta$ and show that the bound cannot be satisfied if $\delta \leq 0$. Let $A = \frac{\gamma}{(1+\gamma)^2}$ and $B = \frac{\gamma}{1+\gamma}$. The above bounds then entail $\frac{2}{9} < A < \frac{1}{4}$ and $\frac{1}{3} < B < \frac{230}{3}$. To eliminate $\beta''$, we rewrite (S.13) as $2\beta''(\alpha^* - 3A)(1+\gamma) = 2\alpha^{*2}\big[(1-\delta)(\alpha^* - \frac{3}{2}B) + (\gamma - 1)\alpha^*\big]$ Notice that $(\alpha^* - 3A) > 0$. Therefore, inequality (S.15) becomes $\alpha^*\big[(1-\delta)(\alpha^* - \frac{3}{2}B) + (\gamma - 1)\alpha^*\big] > 3(\alpha^* - 3A)\big[(1-\delta)(\alpha^* - B) + (\gamma-1)\alpha^*\big]$ Collecting the $1-\delta$ terms on one side gives

$$-2(\gamma-1)\alpha^*(\alpha^* - \frac{9}{2}A) > (1-\delta)\big[3(\alpha^* - B)(\alpha^* - 3A) - (\alpha^* - \frac{3}{2}B)\alpha^*\big] \tag{S.20}$$

The term in the square brackets on the RHS is an increasing function of $\alpha^*$ in the relevant range. Therefore, the term in the square brackets is lower bounded by its value at $\alpha^* = 1$, i.e. $3(1-B)(1-3A) - (1-\frac{3}{2}B)$. This can be seen numerically to be positive over the relevant range. Since the RHS of (S.20) is positive, the LHS must also be positive. By (S.18), $-2(\alpha^* - \frac{9}{2}A) > 0$. Combining this with (S.20) gives $\gamma > 1$. Further, the term inside of the square brackets of (S.20) is positive, so we can get a function of $\gamma$ and $\alpha^*$ which bounds $1-\delta$

$$1-\delta < \frac{-2(\gamma-1)\alpha^*(\alpha^* - \frac{9}{2}A)}{3(\alpha^* - B)(\alpha^* - 3A) - (\alpha^* - \frac{3}{2}B)\alpha^*} \tag{S.21}$$

We will examine this bound by first showing the RHS is a decreasing function of $\alpha^*$ in the relevant range. The derivative of the numerator is $-2(\gamma-1)(2\alpha^* - \frac{9}{2}A)$, which is negative. The derivative of the denominator is $4\alpha^* - 9A - \frac{3}{2}B$, which is positive. Putting these together in the usual quotient rule - along with the already established fact that the numerator and denouement are positive - one sees that the whole derivative is negative. Therefore the right hand side is upper bounded by its value at $\alpha^* = 1$, giving a bound on $1-\delta$

$$1-\delta < \frac{-2(\gamma-1)(1-\frac{9}{2}A)}{3(1-B)(1-3A) - (1-\frac{3}{2}B)} \tag{S.22}$$

Numerically, the RHS has a maximum less than one, contradicting the claim that $\delta < 0$. Therefore, there is no feasible stable stationary state in this case.

**Case 3:** $m_2 = 0$ **&** $m_1 > 0$

We choose as a new characteristic velocity & characteristic force ratio

$$V''' = \frac{m_1 g}{6\pi\mu L} \tag{S.23}$$

$$\beta''' = -\frac{kq_1q_2}{L^2 m_1 g} \tag{S.24}$$

These choices give as a nondimensional dynamic equation

$$\begin{aligned} \dot{\boldsymbol{\alpha}} &= \frac{3}{2|\boldsymbol{\alpha}|^3}\beta''' \boldsymbol{\mathcal{G}} \cdot \boldsymbol{\alpha} - \frac{3}{4}\boldsymbol{\mathcal{G}} \cdot \hat{\mathbf{z}} - \beta''' \frac{(1+\gamma')^2}{\gamma' |\boldsymbol{\alpha}|^3} \boldsymbol{\alpha} \\ &+ (1+\gamma')\hat{\mathbf{z}} \end{aligned} \tag{S.25}$$

This equation is the same as (S.8) with $\delta \to 0$, $\beta'' \to \beta'''$ and $\gamma \to \gamma'$. Therefore there is no feasible vertical stable stationary state in this case.

**Case 4:** $m_2 = m_1 = 0$

If both particles are neutrally buoyant we have as a dimensional dynamic equation

$$\dot{\mathbf{d}} = \frac{1}{8\pi\mu}\left( - \frac{2kq_1q_2}{|\mathbf{d}|^3} \boldsymbol{G} \cdot \mathbf{d} \right) - \frac{1}{6\pi\mu}\left( - \frac{kq_1q_2}{|\mathbf{d}|^3}(\frac{1}{a_1} + \frac{1}{a_2})\mathbf{d} \right)$$

Owing to the rotational symmetry of this system, there is clearly no feasible stable stationary state in this case.

# 2 Necessity And Sufficiency Of Stability Conditions

We now examine formally the local stability conditions for a class of systems that evolve according to equation (9). We will show that (14) - (16) are necessary and sufficient conditions for the stability of equilibria of the form $\boldsymbol{\alpha}^* = \alpha^* \hat{z}$. We denote the relative position of the particles by $\boldsymbol{\alpha} = \alpha_z \hat{\boldsymbol{z}} + \epsilon \hat{\boldsymbol{x}}$. We assume that $\epsilon \ll 1$ so that third and higher order terms in $\epsilon$ of (9) are neglected. In this approximation the dynamics are

$$\dot{\alpha}_z = f(\alpha_z) - \epsilon^2 r(\alpha_z) \tag{S.26}$$

$$\dot{\epsilon} = g(\alpha_z)\epsilon \tag{S.27}$$

where the algebraic form of $f$ and $g$ are given in equations (13) & (12) and the forms of $r$ is

$$r(\alpha_z) \quad = \quad \frac{6\beta}{\alpha_z^5} - \frac{3\beta(1+\gamma)^2}{2\gamma\alpha_z^4} + \frac{3(1-\delta)}{2\alpha_z^3} \tag{S.28}$$

The dynamic equations (S.26) & (S.27) are valid for $\epsilon \ll 1$ and any $\alpha_z$. However, it will become necessary to assume $|\alpha_z - \alpha^*| \ll 1$ to complete the proof. It is important to notice that if $\alpha_z > 0$, then $f(\alpha_z)$ is continuously differentiable and $g$ is continuous in an open neighborhood of a steady state $\boldsymbol{\alpha}^*$.

That equation (14) and inequalities (15) & (16) are necessary for an stable steady state $\boldsymbol{\alpha}^*$ is clear. If equation (14) does not hold, the system isn't even in a steady state. We now move on to the inequalities. Use the fact that, by continuity, if these inequalities hold at $\boldsymbol{\alpha}^*$ then they hold approximately in an open neighborhood of $\boldsymbol{\alpha}^*$. Suppose, for contradiction, one of the inequalities (15) & (16) is violated. If we perturb the system in whichever direction the relevant function is nonnegative, there will not be a restoring force in that direction. This contradicts the claim that the system is stable.

We now check the sufficiency of inequalities (15) and (16). Call a system "locally Lypunov stable" if the so-called Lypunov function $V$ has a root at the given stationary state $\boldsymbol{\alpha}^*$, is positive off of the stationary state and has negative time derivative in an open set around the stationary state. We examine the simple Lypunov function $V(\boldsymbol{\alpha}) = (\boldsymbol{\alpha} - \boldsymbol{\alpha}^*)^2$. This obviously has the desired properties $V(\boldsymbol{\alpha}^*) = 0$ and $V(\boldsymbol{\alpha}) > 0$ if $\boldsymbol{\alpha} \neq \boldsymbol{\alpha}^*$. Taking the non-dimensional time derivative one finds

$$\dot{V}(\boldsymbol{\alpha}) = 2(\alpha_z - \alpha^*)\dot{\alpha_z} + 2\epsilon\dot{\epsilon} \tag{S.29}$$

We will now show that this is negative in an open neighborhood containing $\boldsymbol{\alpha}^*$. We will do so by relating the above equation to the dynamics (S.26) & (S.27). Start with the $\dot{\epsilon}$ term. Combining (S.27) with (S.29), one sees that

$$\dot{V}(\boldsymbol{\alpha}) = 2(\alpha_z - \alpha^*)\dot{\alpha_z} + 2g(\alpha_z)\epsilon^2 \tag{S.30}$$

We now move on to work out the $\dot{\alpha_z}$ term. From (S.26), one finds that (S.30) becomes

$$\dot{V}(\boldsymbol{\alpha}) = 2(\alpha_z - \alpha^*)f(\alpha_z) + 2g(\alpha_z)\epsilon^2 - r(\alpha_z)(\alpha_z - \alpha^*)\epsilon^2 \tag{S.31}$$

Finally we must assume that $\alpha_z$ is approximately $\alpha^*$ so that $(\alpha_z - \alpha^*)\epsilon^2 \approx 0$. Therefore the remainder term $r(\alpha_z)$ disappears and one has

$$\dot{V}(\boldsymbol{\alpha}) = 2(\alpha_z - \alpha^*)f(\alpha_z) + 2g(\alpha_z)\epsilon^2 \tag{S.32}$$

If (15) holds, then the second term is negative. If (14) & (16) holds, then the first term is negative in a neighborhood of $\alpha^*$. This demonstrates the sufficiency of (14) - (16).

Therefore, (14) - (16) are necessary and sufficient conditions for this system to have a locally asymptotically stable configuration at $\alpha^*\hat{\mathbf{z}}$.

# 3 Bounds For Ratio Of Particle Radii When The Particles Are In Feasible Stable Stationary States

We will now show that in the $m_1 > 0$ and $m_2 > 0$ case there are stable configurations only if the higher particle 2 is larger in radius than the lower particle 1 - i.e. the ratio of radii $\gamma = \frac{a_1}{a_2} < 1$. This will be a proof by contradiction. We will start by showing that there cannot be a solution when $\gamma = 1$. Following this, we will establish that if $\gamma > 1$ then a feasible, asymptotically stable steady state does not exist.

## 3.1 Radii Cannot Be Equal

By way of contradiction, assume both $\gamma = 1$ and there exists at least one feasible attractive steady state configuration $\boldsymbol{\alpha}^* = \alpha^* \hat{\boldsymbol{z}}$. We can now write (14) as

$$f(\alpha^*) = (4\alpha^* - 3)((\delta - 1)\alpha^{*2} - 2\beta) = 0. \tag{S.33}$$

The first term cannot be zero because of the feasibility condition (17). By inequality (18), we know that $\beta > 0$. Therefore, $\alpha^{*2} = \frac{2\beta}{\delta - 1}$. Therefore in order for a feasible stable steady state to exist in the $\gamma = 1$ case, one must have $\delta > 1$. Take the derivative of (S.33) to find

$$f'(\alpha^*) = 4((\delta - 1)\alpha^{*2} - 2\beta) + 2(\delta - 1)\alpha^*(4\alpha^* - 3) \tag{S.34}$$

The first term is zero by (S.33) and the second term is positive by $\delta > 1$ & (17). This contradicts inequality (16). Therefore, there cannot be a feasible stable stationary state in this case.

## 3.2 Upper Particle Cannot Be Smaller Than The Lower One In Feasible Stable Steady State

We move on to the $\gamma > 1$ case. We will use proof by contradiction, supposing that we have a set $\alpha^*$, $\beta$, $\delta$, $\gamma$ where $\gamma > 1$ and conditions (14) - (17) obtain. Recall that $\beta$ and $\delta$ must both be positive by inequalities (18) & (19). We will start the demonstration by showing that $\gamma > 1$ implies that $\delta > 1$. Then we will show that conditions (14) and (15) combine in a way that contradict condition (17).

We start by taking advantage of the fact that, by equation (14) and inequalities (15) (17), $f(\alpha^*) - \alpha^* g(\alpha^*) > 0$. Simplifying, we find

$$(1 - \delta)(3\gamma - 4\alpha^*(1 + \gamma)) - 4\alpha^*(\gamma^2 - 1) > 0 \tag{S.35}$$

Because of condition (17), $3\gamma - 4\alpha^*(1 + \gamma) < 0$. Further, if $\gamma > 1$, then $\gamma^2 > 1$ so the second term is negative. Therefore, in order for the above relation to hold, $\delta > 1$.

Now that we have $\delta > 1$, we aim toward eliminating $\beta$ by writing (14) as

$$-2\beta(1+\gamma)^2(\alpha^* - \frac{3\gamma}{(1+\gamma)^2}) = \left(2(\gamma-\delta)(1+\gamma)\alpha^* + 3\gamma(\delta-1)\right)\alpha^{*2} \quad \text{(S.36)}$$

The left hand side is negative, therefore the right hand side must be negative, in other words

$$(\gamma-1)\alpha^* < (\delta-1)(\alpha^* - \frac{3}{2}\frac{\gamma}{1+\gamma}) \quad \text{(S.37)}$$

Because $\gamma > 1$, the left hand side is positive. Therefore, $\alpha^* > \frac{3}{2}\frac{\gamma}{1+\gamma}$. We now use equation (S.36) to eliminate $\beta$ from (16). This gives that

$$(\delta-1)\left(2\alpha^{*2} - \frac{3\gamma(7+\gamma)}{2(1+\gamma)^2}\alpha^* + \frac{9\gamma^2}{(1+\gamma)^3}\right) < 2(\gamma-1)\alpha^*(\alpha^* - \frac{9\gamma}{2(1+\gamma)^2}) \quad \text{(S.38)}$$

The left hand side must be positive or non positive. Because $\delta > 1$, if the the left hand side in the above inequality is positive, then one can combine the above with (S.37). Simplifying, one finds $\alpha^* < \frac{3\gamma}{(1+\gamma)^2}$ which violates condition (17). Therefore the left hand side must be nonpositive:

$$2\alpha^{*2} - \frac{3\gamma(7+\gamma)}{2(1+\gamma)^2}\alpha^* + \frac{9\gamma^2}{(1+\gamma)^3} \leq 0 \quad \text{(S.39)}$$

Notice that if $\alpha^*$ is very large then the polynomial in (S.39) is positive and, speaking formally, if $\alpha^* = 0$ it is also positive. Therefore the above can only be negative for $\alpha^* > 1$ if the polynomial has two distinct positive real roots. We now look at the discriminant, which must be positive for the roots to be real and distinct

$$0 < \Delta = \frac{9\gamma^2(\gamma-1)(\gamma-17)}{4(1+\gamma)^4} \quad \text{(S.40)}$$

We therefore have $\gamma > 17$. Further, notice that the only negative term in (S.39) is the middle term. Therefore, we have

$$\alpha^{*2} + \frac{9\gamma^2}{2(1+\gamma)^3} \leq \frac{3\gamma(7+\gamma)}{4(1+\gamma)^2}\alpha^* \quad \text{(S.41)}$$

$$\alpha^* < \frac{3\gamma(7+\gamma)}{4(1+\gamma)^2} \quad \text{(S.42)}$$

But right hand side in (S.42) is less than 1 for all $\gamma > 17$. This is a contradiction to condition (17). Therefore conditions (14) & (16) and condition (17) cannot be simultaneously satisfied if $\gamma > 1$. Thus we have $\gamma \leq 1$.

### 3.3 Conclusion

We have established $\gamma \neq 1$ and that $\gamma \leq 1$. This establishes that $\gamma < 1$, that the upper particle in the feasible stable steady state must have a larger radius than the lower particle.
